# Supplementary material for: PTCMIL: Multiple Instance Learning via Prompt Token Clustering for Whole Slide Image Analysis
Source: arXiv:2507.18848 source file (2025-07-24)
Supplement: Supplementary file 1 [file 07-appendix.tex]

In the Appendix, we provide five sections for supplementary information and experimental results. In Appendix~\ref{appendix:baselines}, we offer a detailed description of the baseline implementation and the specific hyperparameters used in each baseline. 
In Appendix~\ref{appendix:feature_ablation}, we provide the result with foundation model features to show SMILE is effective even with advanced features.
In Appendix~\ref{appendix:advanced_vit_student_model}, we provide the ablation study on different ViT student model architectures to show that SMILE can further improve the classification performance with advanced ViT structures.
In Appendix~\ref{appendix:tl_analysis}, we justify the reason that self-attention-based ViT structure is more suitable to be used as token labelers.
Finally, in Appendix~\ref{appendix:code_and_dataset}, the source code of SMILE and links to the public datasets are included.

\section{Datasets}

\section{Baseline Implementations}

\label{appendix:baselines}
% Since the batch size is set to 1 for MIL problem, the order in which the data is trained significantly affects performance. Therefore, we meticulously control even the order of the training data for different methods. 
% We provide the implementation details of feeding the same training set, validation set and testing set of ours to baselines here. \\
In this section, we provide the implementation details of baselines under the same experimental settings as ours, using an identical training, validation, and testing set. 

For ABMIL \cite{ilse2018attention}, we employ the gated-attention mechanism as suggested in the original paper, which is a permutation-invariant aggregation operator. 
We strive to maintain the model structure as proposed by the original paper. 
~The source code of ABMIL: \url{https://github.com/AMLab-Amsterdam/AttentionDeepMIL}.

For DSMIL \cite{li2021dual}, a dual-stream multiple instance learning network is proposed to aggregate the patch embedding. 
It uses a two-stream architecture to learn a patch and a slide classifier, including a max-pooling branch and an aggregation branch. The max-pooling is used to predict the slide-level label, and the selected patch is called critical instance. Then, the aggregation branch measures the distance of all instances and the critical instance. The distances are used as weights for all instances to generate another slide-level prediction score. The scores of the two streams are averaged to generate another slide-level prediction score.
In this work, we focus on the improvement of aggregation, thus we use our features as the input to DSMIL. The source code of DSMIL: \url{https://github.com/binli123/dsmil-wsi}.

CLAM \cite{lu2021data} propose a clustering-constrained-attention multiple-instance learning MIL framework. Instead of only using the attention mechanism, it also involves the instance-level clustering based on in-the-class attention and out-the-class attention scores. A hyperparamter B controls the selected patch number with highest and lowest attention scores. We follow the original implementation, setting B to 8. Additionally, the final optimization function is a weighted summation of bag-level classification loss and instance-level smooth SVM clustering loss. A hyperparameter to control the proportion of bag-level loss term, which is set to 0.7, which is also the same as the original implementation.
The source code of CLAM \cite{lu2021data}: \url{https://github.com/mahmoodlab/CLAM}.

For TransMIL \cite{shao2021transmil}, we conduct experiments on embedding dimensions of not only 512 as suggested in the original paper, but also 384, and report better results in our paper. TransMIL has unique sinusoidal encoding and conditional position encoding in its PPEG block between two Transformer blocks. We keep using the same convolutional layers proposed in the original paper. 
The source code of TransMIL: \url{https://github.com/szc19990412/TransMIL}.

DTFD \cite{zhang2022dtfd} proposes a double-tire feature distillation framework based on ABMIL. At the begining, it randomly splits patches in one WSI into several pseudo bags. In the Tier-1 ABMIL, the optimization cross-entropy function calculates the loss between slide label and predicted instance labels within each pseudo bag. In the Tier-2 ABMIL, the optimization cross-entropy function calculates the loss between slide label and predicted pseudo bag labels. The final optimization function is the average of two tiered optimization function. The hyperparameter numGroup controls the bag number. We follow the original implementation, setting it as 5. The source code of DTFD: \cite{tang2023multiple}: \url{https://github.com/hrzhang1123/DTFD-MIL}.

% For MHIM \cite{tang2023multiple}, we compare to the model with TransMIL backbone. 
MHIM \cite{tang2023multiple} proposes a masked hard instance mining strategy. It includes high attention masking (HAM) that can be combined with low attention masking (L-HAM), random attention attention masking (R-HAM), and low-and-random attention masking (LR-HAM). These masking strategies are controlled by four hyperparameters: mask ratios for random attention masking, high attention masking, low attention masking and high-random attention masking.
They are set as provided in the original GiuHub Repository with the TransMIL backbone. 
% The mask ratio decay strategy is used with hyperparameter mrh\_sche. 
Another hyperparameter for controlling the consistency loss in the optimization function, which is set to 0.1 according to the original implementation. 
We also keep the same hyperparameters of exponential moving average\,(EMA) to update teacher and student model parameters as in the original paper. 
% We keep the same hyperparameters mm, mm\_sche, used for exponential moving average (EMA) to update teacher and student model parameters as in the original paper. 
The source code of MHIM: \url{https://github.com/DearCaat/MHIM-MIL}.

\section{Ablation Study on $\alpha$}

\section{Ablation Study on CTransPath Features}
\label{appendix:ctranspath_features}
Following many baselines involved in our study, such as \cite{lu2021data,zhang2022dtfd,shao2021transmil}, we used a ResNet50 pretrained on ImageNet as the feature extractor to generate features for patch instances from WSIs. To demonstrate the generalizability of the proposed SMILE framework on more advanced feature extractors, in this section, we report the results of using CTransPath features. CTransPath \cite{wang2022transformer} is a foundation pathology image model with combined ViT and CNN as backbones. It is pretrained on around 15 million patches from nine datasets, including Camelyon16 and TCGA-lung, with MoCo v3 \cite{he2022masked}. 
% Most patches for pretraining are of 20$\times$ magnification.
We evaluate the performance of SMILE and the baselines using features generated from CTransPath. For CTransPath, patch instances are extracted at 20$\times$ magnification to generate features in order to improve the efficiency of model training. Table \ref{tab:advanced_features} summarizes the performance when combining features generated from CTransPath with MIL aggregators for Camelyon16 and TCGA-NSCLC datasets. Comparing Table \ref{tab:baselines} and \ref{tab:advanced_features}, we can observe an enhancement in performance of SMILE and all baselines when using more advanced features. Particularly, SMILE demonstrates superior performance over the baselines for both Camelyon16 and TCGA-NSCLC datasets, indicating that SMILE serves as a feature-agnostic and robust MIL aggregator.

\section{Ablation Study on Advanced ViT Student Models}
\label{appendix:advanced_vit_student_model}
We used Vanilla ViT as our student backbone model. Given GPU capacity constraints, there are limitations to the structure of ViT in handling 256 $\times$ 256 size patches extracted at a magnification of 40$\times$. However, by reducing the magnification or increasing patch size to decrease the number of patch instances, we can utilize more advanced ViT architectures as student backbone models. As an extension in Sec. \ref{appendix:feature_ablation}, we applied SMILE to advanced ViT backbones, CaiT\cite{touvron2021going} and CRATE\cite{yu2024white}, using features extracted with CTransPath at the magnification of 20$\times$. However, due to GPU memory constraints, we set the head count to 1 and the embedding dimension to 192. Table \ref{tab:advanced_vit_stduent} demonstrates the performance change when applying SMILE to CaiT and CRATE on the Camelyon16 and TCGA-NSCLC datasets. 
Considering the head is set to 1, both CaiT and CRATE exhibit comparable performance when compared to the vanilla ViT. 
Particularly, CRATE significantly outperforms the existing MIL aggregator baselines when used with SMILE on both Camelyon16 and TCGA-NSCLC. In conclusion, SMILE demonstrates its capability as a training objective that can elevate the potential performance of ViT as an MIL aggregator.

\input{table/stduent_vit_ablation}

\section{Code and Data Availability}
\label{appendix:code_and_dataset}
The source code of SMILE: \url{https://anonymous.4open.science/r/SMILE} \\
Camelyon16 dataset:~\url{https://camelyon16.grand-challenge.org}.\\
TCGA-NSCLC dataset:~\url{https://portal.gdc.cancer.gov} \\
