# Supplementary material for: PTCMIL: Multiple Instance Learning via Prompt Token Clustering for Whole Slide Image Analysis
Source: arXiv:2507.18848 source file (2025-07-24)
Supplement: Supplementary file 2 [file appendix_classification.tex]

\begin{table*}[!ht]
\centering
\caption{Classification result of PTCMIL on Camelyon16 and TCGA-NSCLC datasets (ResNet50 feature). AUC and Accuracy are reported. Bold highlights the best performance. {\footnotesize ($*$: Unable to reproduce performance from the provided code even with our best fold performance, we use the paper's reported result.)}} 
\label{tab:appendix_main}
\resizebox{\textwidth}{!}{%
\begin{tabular}{@{}c|c|cc|cc|c|c@{}}
\toprule
\multirow{2}{*}{\makecell{Feature\\extraction}} & \multirow{2}{*}{Method} & \multicolumn{2}{c|}{Camelyon16} & \multicolumn{2}{c|}{TCGA-NSCLC} & \multicolumn{1}{c|}{PANDA} & \multicolumn{1}{c}{\makecell{PANDA $\to$ \\ in-house \\ prostate dataset}} \\ 
\cline{3-8} 
\multicolumn{1}{c|}{} & \multicolumn{1}{c|}{} & AUC & Acc & AUC & Acc & Cohen's $\kappa$ & Acc \\ 
\midrule
\multirow{10}{*}{ResNet50}
& Mean-pooling & $56.27_{5.18}$& $67.71_{1.19}$ & $87.35_{5.89}$ & $80.38_{6.21}$ & $0.633$ & $0.775$ \\ 
& Max-pooling & $90.23_{10.76}$ & $83.28_{9.77}$ & $89.12_{2.13}$ & $80.60_{2.83}$  & $0.374$ & $ 0.612$ \\ 
& ABMIL (NeurIPS'18) \cite{ilse2018attention} & $84.84_{5.57}$ & $85.94_{4.76}$ & $89.10_{0.80}$ & $81.42_{1.58}$ & $0.730$ & $0.775$ \\ 
& DSMIL (CVPR '21) \cite{li2021dual} & $85.46_{2.70}$ & $81.77_{1.19}$ & $93.56_{1.03}$ & $86.64_{1.82}$ & $0.771$ & $0.562$\\ 
& CLAM (Nat. Biomed. Eng. '21) \cite{lu2021data} & $91.57_{1.29}$ & $88.02_{1.63}$ & $92.99_{2.16}$ & $85.66_{2.16}$ & $0.770$ & $0.694$\\ 
& TransMIL (NeurIPS'22) \cite{shao2021transmil} & $92.58_{2.84}$ & $86.46_{1.80}$ & $92.28_{2.12}$ & $83.87_{3.22}$ & $0.777$ & $0.766$ \\ 
% & DTFD-MIL (CVPR'22) \cite{zhang2022dtfd} & $93.75_{0.98}$ & $90.11_{3.69}$ & $94.10_{1.83}$ & $86.70_{0.68}$ & $0.800$ & $0.802$ \\ 
& ILRA (ICLR'23) \cite{xiang2023exploring} & $92.78^{*}$ & $89.92^{*}$ & $91.71_{1.89}$ & $84.40_{2.57}$ & $0.815$ & $0.828$ \\ 
& PANTHER (CVPR'24) \cite{Song_2024_CVPR} & $58.15_{9.14}$ & $62.17_{0.35}$ & $75.01_{1.78}$ & $65.58_{2.22}$ & $0.182$ & $0.214$ \\ 
& MambaMIL (MICCAI'24) \cite{yang2024mambamil} & $77.75_{4.79}$ & $79.84_{3.14}$ & $94.10_{4.63}$ & $\mathbf{87.40_{1.61}}$ & $0.810$ & $0.805$\\ 
& PTCMIL (ours) & $\mathbf{95.35_{1.77}}$ & $\mathbf{90.63_{3.66}}$ & $\mathbf{94.59_{0.53}}$ & $87.25_{1.11}$ & $\mathbf{0.825}$ & $\mathbf{0.865}$ \\ 
\bottomrule
\end{tabular}%
}
\end{table*}
